# Supplementary material for: A 3D generative model of pathological multi-modal MR images and segmentations
Source: arXiv:2311.04552 source file (2023-11-08)
Supplement: Supplementary file 1 [file paper09_dgm4miccai_crv_SUPPLEMENTARY.pdf]

## A Training hyperparameters and augmentations

Table 1: Label and image generator hyperparameters

| Variational autoencoder |                     |                                           |                                        |
|-------------------------|---------------------|-------------------------------------------|----------------------------------------|
| Loss weights            |                     | Other parameters                          |                                        |
| Patch GAN loss          | 0.1                 | epochs                                    | 250                                    |
| KLD loss                | $10^{-8}$           | train time                                | 4h38 min                               |
| reconstruction loss     | 1.0                 | optimiser                                 | Adam                                   |
| perceptual loss         | 10                  | learning rate                             | vae: $2 \cdot 10^{-4}$ disc: $10^{-4}$ |
| hardware                | NVIDIA DGX A100     | batch size                                | 8                                      |
| Latent diffusion model  |                     |                                           |                                        |
| epochs                  | 400                 | training time                             | 12h                                    |
| warm-up learning rate   | $10^{-8}$           | batch size                                | 8                                      |
| base learning rate      | $2.5 \cdot 10^{-5}$ | loss                                      | $l_1$                                  |
| perceptual loss         | 10                  | hardware                                  | NVIDIA DGX A100                        |
| Image generator         |                     |                                           |                                        |
| Epochs                  | 350                 | training time                             | 2 weeks                                |
| hardware                | single A100 GPU     | optimiser                                 | Adam                                   |
| learning rate           | $2 \cdot 10^{-4}$   | number of discriminator                   | 3                                      |
| Loss weights            |                     |                                           |                                        |
| Generator               |                     | Discriminator                             |                                        |
| KLD                     | $10^{-5}$           | feature loss                              | 0.25                                   |
| perceptual loss         | 1.5                 | <b>gen. and disc. training thresholds</b> |                                        |
| slice consistency       | 0.5                 | lower (D only)                            | 0.65                                   |
| perceptual loss         | 10                  | lower (G only)                            | 0.75                                   |

Augmentations were implemented using MONAI (<https://monai.io/>).

Table 2: Transformations applied to the different modules. The intensity transforms, marked with (\*) were only applied to images, not labels.

| Augmentation               | VAE (ranges)                                                                      | DM (ranges)                                                                    | Image generator (ranges)                                                          |
|----------------------------|-----------------------------------------------------------------------------------|--------------------------------------------------------------------------------|-----------------------------------------------------------------------------------|
| Random affine              | rotation: [-0.05, 0.05], shear: [0.001, 0.05], scale:[0, 0.05], probability: 0.15 | rotation: [-0.1, 0.1], shear: [0.001, 0.15], scale:[0, 0.3], probability: 0.15 | rotation: [-0.05, 0.05], shear: [0.001, 0.05], scale:[0, 0.05], probability: 0.33 |
| Random bias field (*)      | -                                                                                 | -                                                                              | intensity: (0, 0.005), probability: 0.33                                          |
| Random Gaussian noise (*)  | -                                                                                 | -                                                                              | mean: 0.0, $\sigma$ range: [0.005, 0.015], probability: 0.33                      |
| Random contrast adjust (*) | -                                                                                 | -                                                                              | $\gamma$ range: [0.9, 1.15], probability: 0.33                                    |

## B Additional result figures

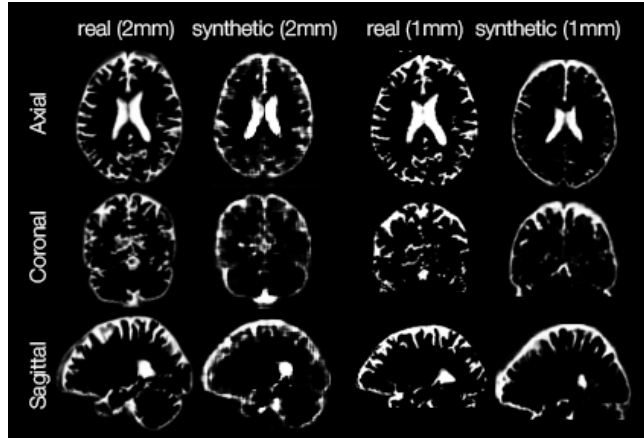

Fig. 1: Example CSF real and synthetic label channels for both the  $1mm^3$  and  $2mm^3$  models, showing the loss of detail in the subarachnoid space CSF on the  $1mm^3$  model. All images are unpaired.

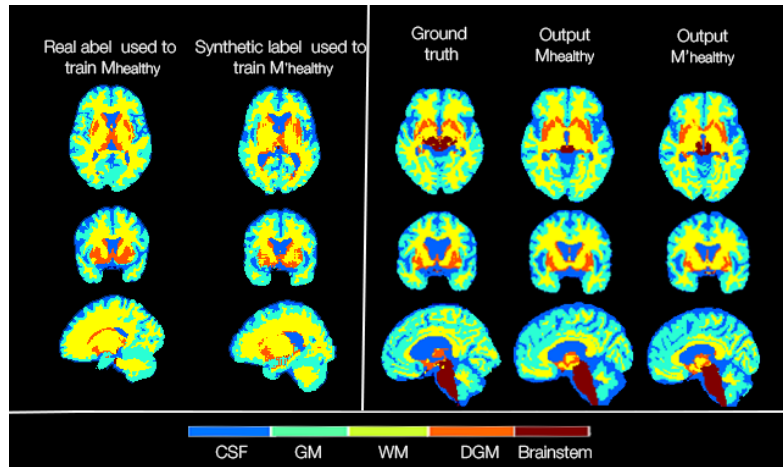

Fig. 2: From left to right: example real label from our private dataset used to train model  $M_{healthy}$  (see section 3.1), synthetic healthy label generated by our model used to train  $M'_{healthy}$ , ground truth sample from the test set of the private dataset and corresponding  $M_{healthy}$  and  $M'_{healthy}$  outputs. Examples shown are for the  $2mm^3$  model.
